# Supplementary material for: Coherent Interactions Between Silicon-Vacancy Centers in Diamond
Source: arXiv:2105.01103 ancillary file (2021-05-03)
Supplement: Supplementary file 1 [file Supplemental.pdf]

# Supplementary Information for Coherent Interactions Between Silicon-Vacancy Centers in Diamond

Matthew W. Day,[1] Kelsey M. Bates,[1] Christopher L. Smallwood,[2,1] Rachel C. Owen,[1] Tim Schröder,[3] Edward Bielejec,[4] Ronald Ulbricht,[5] and Steven T. Cundiff[1,*]

[1]*Department of Physics, University of Michigan, Ann Arbor, MI 48109, USA*

[2]*Department of Physics, San José State University, San Jose, CA 95192, USA*

[3]*Department of Physics, Humboldt-Universität zu Berlin, Newtonstraße 15, 12489 Berlin, Germany*

[4]*Sandia National Laboratories, Albuquerque, NM 87185, USA*

[5]*Max Plank Institut für Polymerforschung, Ackermannweg 10, 55128 Mainz, Germany*

(Dated: April 21, 2021)

Here we elaborate on a few details which are crucial to reproducing our work and understanding our results in the main text. First, we add a few details about the sample preparation. Next, we show a DQ2D spectrum for both excitation polarizations, for completeness. Then we flesh out the point made in the main text that all 2Q peaks are the result of Louiville pathways reducible to sums of sets of pathways corresponding to pairs of coupled two-level systems. Finally, we add a bit of detail to the comparison between our qualitative model for the pump-2Q2D probe experiment and the data, and address the crucial detail that our pump pulse was comparable in spot-size to the FWM probe pulses.

## SAMPLE DETAILS

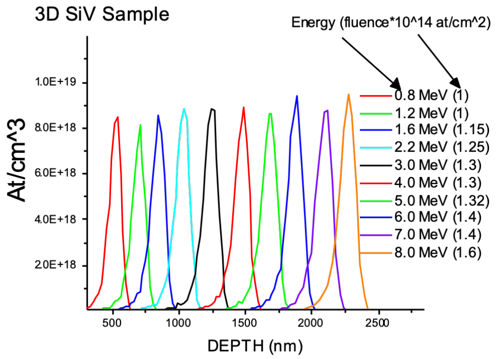


FIG. 1. The detailed focussed-ion beam implantation parameters for the sample.

The sample studied in this Letter was a Type-IIa diamond purchased from Element Six. The sample was implanted in four roughly equally sized patches, covering the sample surface which was $\sim$ 2mm $\times$ 2mm across, with a thickness of 0.3mm. Silicon-29 atoms were implanted with densities and implantation depths detailed in Figure 1. Following this, the sample was annealed at $1000-1050°$C and an anti-reflective coating was applied to reduce the effect of the index mismatch between diamond and vacuum on the collection efficiency of fluorescence from the color centers.

## COMPLETE SET OF DOUBLE-QUANTUM SPECTRA

The above DQ2D spectra show that all states which can be excited by our experiment have excitation-dependent interactions with both their resonant and non-resonant counterparts

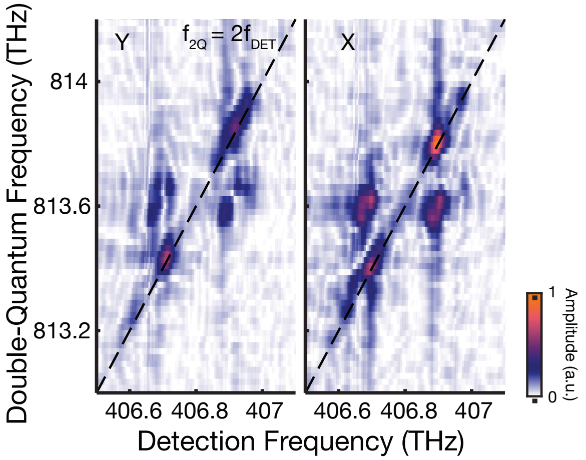


FIG. 2. A complete set of double-quantum, two-dimensional spectra taken with excitation pulses polarized in both the X and Y (with respect to the experimental apparatus) directions.

in other color centers.

## PAIR-WISE RABI OSCILLATION DETAILS

In the main text, we argue that the main cause of the oscillation behavior seen when conducting pump-2D probe measurements on our sample is pair-wise Rabi oscillations of coupled two-level systems. Here we elaborate on two details of our qualitative model. First, we illustrate in more detail the assertion that peaks in the 2Q2D spectra are simply just a superposition of pairwise, joint two-level system coupling. In Figure 3(a), we show a simulated 2Q2D spectrum for just one pair of resonant two-level systems coupled together with bare, linear transition frequency 406.9 THz. When we take the relevant energy level system for calculating our 2Q2D spectrum, shown in Figure 3 and as detailed in Fig. 1 in the main text. For the in-plane oriented centers, transitions B and C are responsible for the highest signal-to-noise ratio peaks in the X-polarized 2Q2D spectra. Spin-orbit coupling and the selection rules for transitions between the few-body electron states constituting the zero-phonon line yield two pairs of transitions arising from four distinct eigenstates of the system [1], which can either couple together resonantly (green and blue boxes) or non-resonantly (orange and brown boxes).

As illustrated in Figure 3(b), this situation yields a spectrum that is simply a superposition of four separate pairs of two-level systems which interact (as denoted by the separated

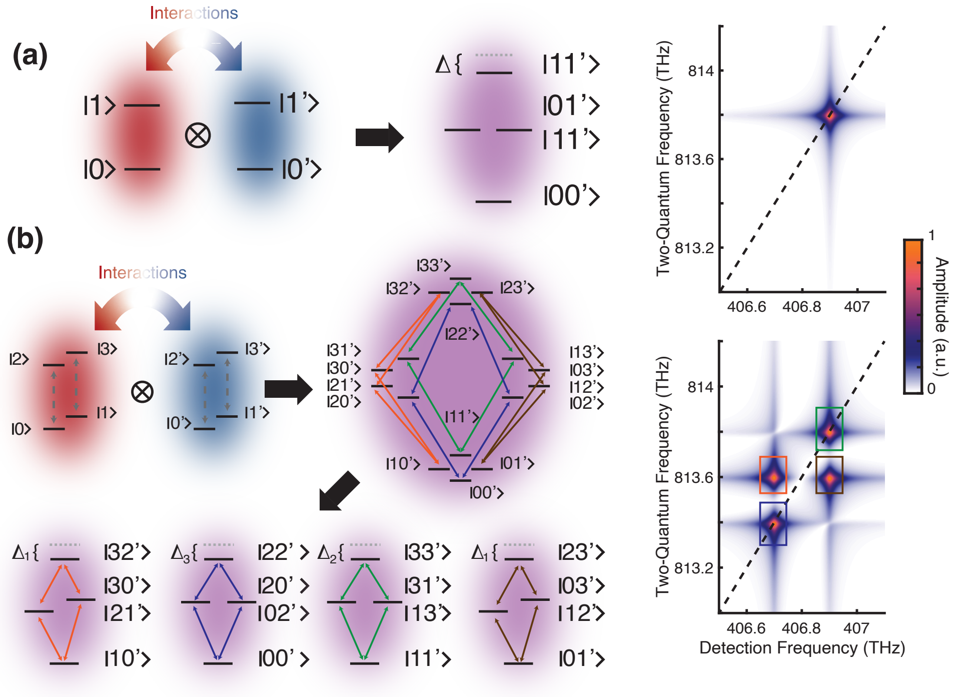


FIG. 3. (a) The simulated spectrum from just one pair of resonant two level systems coupled together through interactions. (b) The simulated spectrum for a pair of systems with the relevant energy level diagrams for the $SiV^-$ system. The spectrum is the sum of the contributions from the four possible combinations of two level systems, whose optical transitions are denoted with color-coded arrows corresponding to the boxed peaks in the simulated 2Q2D spectrum. .

systems and color-coded transitions). Following the conventions in [2], we simulate the 2Q2D spectrum arising from each of the separate situations, finding that the spectrum in Figure 3(b) is simply the superposition of four separate peaks of the form detailed in the main text, equation 1. To simulate the spectra, we use transition frequencies 406.7 and 407.9 with linewidths of 12 GHz, corresponding roughly to the experimentally measured spectra in the main text. Our method of separating out peaks for fitting is justified by the particular form of the energy level scheme in the $SiV^-$ center, but can be easily generalized to systems with more complex level systems or coupling between split ground or excited states. We denote the non-resonant interaction parameter $\Delta_1$ and the resonant interaction parameters are denoted $\Delta_2$ and $\Delta_3$ in Fig. 3.

For the pump, 2Q2D probe measurements, we took slightly lower resolution spectra to speed up acquisition time (as each full set of 2D spectra took roughly 20-30 hours to acquire)

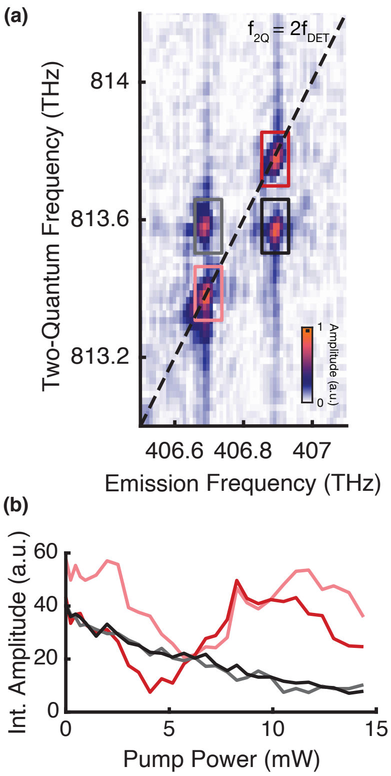


FIG. 4. (a) One pump-2D probe spectra with the integrated peaks box bounds displayed. (b) The full set of integrated pump-2D probe peaks showing the dramatic difference between resonant and non-resonant 2Q peaks.

by continuously scanning the second time delay. The boxes denoted in Figure 2(c) in the main text correspond to the integrals of the peaks of the lower resoultion datasets whose exact bounds are denoted in the boxes in Figure 4. As can be seen, this set of data was relatively lower quality than the spectra presented in the second Figure in the main text. In Figure 2 in the main text, the spectral resolution was no better than 20 GHz in the double-quantum frequency direction, and no better than 4 GHz in the detection direction. The resolution of the spectra taken in the pump, DQ2D probe experiment presented in Figure 4 was nominally similar (not better than 20 GHz in the double-quantum direction, and not better than 5 GHz in the detection direction) but because the second time delay was swept continuously while acquiring spectra, the signal-to-noise ratio of those spectra was functionally worse. In the high-quality, main text spectra, the time-domain signal-to-noise (SNR) ratio was 6, leading to a frequency-domain of roughly 13. In the pump, DQ2D probe data, the *maximum* SNR was roughly 8 in the frequency domain and between 3 and 4 in

the time domain, slightly degrading the resolution of the resulting DQ2D spectra.

Finally, in the main text we fit the lineshape of the peak corresponding to the transition at 406.9 THz, yielding an estimation for the power required to flop a pair of centers into the excited state. Counter-intuitively, a $\pi$-pulse retains its meaning in this particular physical situation. To see that this is true, take the joint two-level system representing a joing pairwise two-level system under a driving field

$$H = \begin{pmatrix} \epsilon_{00'} & -\vec{\mu}\cdot\vec{E}(t) & -\vec{\mu}\cdot\vec{E}(t) & 0 \\ -\vec{\mu}\cdot\vec{E}(t) & \epsilon_{10'} & 0 & -\vec{\mu}\cdot\vec{E}(t) \\ -\vec{\mu}\cdot\vec{E}(t) & 0 & \epsilon_{01'} & -\vec{\mu}\cdot\vec{E}(t) \\ 0 & -\vec{\mu}\cdot\vec{E}(t) & -\vec{\mu}\cdot\vec{E}(t) & \epsilon_{11'} \end{pmatrix}. \tag{1}$$

We assume that $\epsilon_{00'} = 0$, $\epsilon_{10'} = \epsilon_{10'} = \hbar\omega_1$, $\epsilon_{10'} = 2\hbar\omega_1$, and $\vec{E}(t) = \vec{E}_0\cos(\omega t)$ where $\omega$ is the driving frequency of the field. Using the time-dependant Schrödinger equation, with complex coefficients $c_{ij}$ for each eigenstate, we have the coupled set of differential equations for the time evolution of the system

$$i\dot{c_{00'}}(t) = -\vec{\mu}\cdot\vec{E}_0(c_{10'}(t) + c_{01'}(t))\cos(\omega t) \tag{2}$$

$$i\dot{c_{10'}}(t) = -\vec{\mu}\cdot\vec{E}_0(c_{00'}(t) + c_{11'}(t))\cos(\omega t) + \hbar\omega_1 c_{10'}(t) \tag{3}$$

$$i\dot{c_{01'}}(t) = -\vec{\mu}\cdot\vec{E}_0(c_{00'}(t) + c_{11'}(t))\cos(\omega t) + \hbar\omega_1 c_{01'}(t) \tag{4}$$

$$i\dot{c_{11'}}(t) = -\vec{\mu}\cdot\vec{E}_0(c_{10'}(t) + c_{01'}(t))\cos(\omega t) + 2\hbar\omega_1 c_{11'}(t). \tag{5}$$

The rotating wave approximation consists of making the substitution $d_{00'}(t) = c_{00'}(t)$, $d_{10'}(t) = c_{10'}(t)e^{i\omega t}$, $d_{01'}(t) = c_{01'}(t)e^{i\omega t}$, and $d_{11'}(t) = c_{11'}(t)e^{2i\omega t}$ and throwing away terms that evolve at $2\omega$. Under this approximation, the above set of differential equations becomes

$$i\dot{d_{00'}}(t) = -\frac{\Omega}{2}(d_{10'}(t) + d_{01'}(t)) \tag{6}$$

$$i\dot{d_{10'}}(t) = -\frac{\Omega}{2}(d_{00'}(t) + d_{11'}(t)) + \hbar(\omega - \omega_1)d_{10'}(t) \tag{7}$$

$$i\dot{d_{01'}}(t) = -\frac{\Omega}{2}(d_{00'}(t) + d_{11'}(t)) + \hbar(\omega - \omega_1)d_{01'}(t) \tag{8}$$

$$i\dot{d_{11'}}(t) = -\frac{\Omega}{2}(d_{10'}(t) + d_{01'}(t)) + 2\hbar(\omega - \omega_1)d_{11'}(t) \tag{9}$$

where $\Omega$ is the Rabi frequency $\Omega = \vec{\mu}\cdot\vec{E}/\hbar$. If we assume resonant driving of the system,

then the coefficients for the time-evolution of the four states are

$$d_{00'}(t) = \cos^2(\frac{\Omega t}{2}) \tag{10}$$

$$d_{10'}(t) = d_{01'}(t) = \frac{i}{2}\sin(\Omega t) \tag{11}$$

$$d_{11'}(t) = -\sin^2(\frac{\Omega t}{2}). \tag{12}$$

In our model, we are assuming that the FWM signal strength ($S^{(3)}(\tau, \omega_T, \omega_t)$) depends on the ground state population and resonant interactions ($\Delta$) depend on the excited-state population. From the above derivation, if we assume that we have an ensemble of N systems, then

$$\rho_{00} = N\cos^4(\frac{\Omega t}{2}) \tag{13}$$

and

$$\rho_{11'} = N\sin^4(\frac{\Omega t}{2}) \tag{14}$$

The point here is twofold: one, we have a slightly different scaling of our interactions in the pair-wise scenario than in an ensemble of single, non-interacting two-level systems. Second, although we have a slightly different scaling with pulse area, the meaning of a $\pi$-pulse is the same given that the classic $\sin^2(\Omega t/2)$ and $\cos^2(\Omega t/2)$ behavior is replaced with $\sin^4(\Omega t/2)$ and $\cos^4(\Omega t/2)$ which have the same minima and maxima as the canonical two-level system population coefficients. A final note: this toy model preserves the fact that there is an effective enhancement Rabi frequency (by a factor of two) for the singly excited state because one cannot differentiate between singly excited states *a priori*, just like in the atomic case.

One detail in the fitting not discussed in the main text is that we fixed linewidths in the $T$ direction to be $\gamma_T = 0.021$ THz and $\gamma_t = 0.012$ THz, measured from Lorentzian fits of slices of the peaks at their center energies. We allowed only $\Delta(E)$, $E_\pi$, and the overall amplitude to vary while fitting the real and complex parts of the data simultaneously.

## DETAILS REGARDING SPOT SIZE EFFECTS ON RABI OSCILLATIONS

One final detail not treated in the main text that is important to the overall interpretation of our fit is the following: the pump spot size is the same as that of the four-wave mixing probe beams. One might think that this completely destroys the possibility that *any* Rabi-like behavior wold be observed. This is simply untrue. What *does* happen is that the spatial

inhomogenaiety of the field translates to an apparent reduction in overall Rabi frequency and reduced fringe visibility with increasing pulse area. Figure 5 is a simulation of this phenomena detailing what happens to the apparent Rabi oscillations in the case of similar pump and probe spot sizes.

To create this simulation, we generated a distribution of Rabi frequencies which depended on the pump intensity profile which was measured to be roughly Gaussian with $\sigma_{pump} = 1.33\ \mu$m while the four-wave-mixing probe beams were collinear and also roughly Gaussian with $\sigma_{FWM} = 1.6\ \mu$m. This may look like a hopeless situation for observing Rabi-like behavior, but because the flopping behavior depends on the field and the four-wave-mixing signal depends on the square of the intensity, the signal comes from a spatially more confined spot. We populate the pump spot with a distribution of dipole moments scaled to the pump field, and then calculate the 'effective population fraction' as the fraction of centers in the excited state as a function of pulse area *as seen by the four-wave-mixing probe.* The results of this simulation are presented in 5.

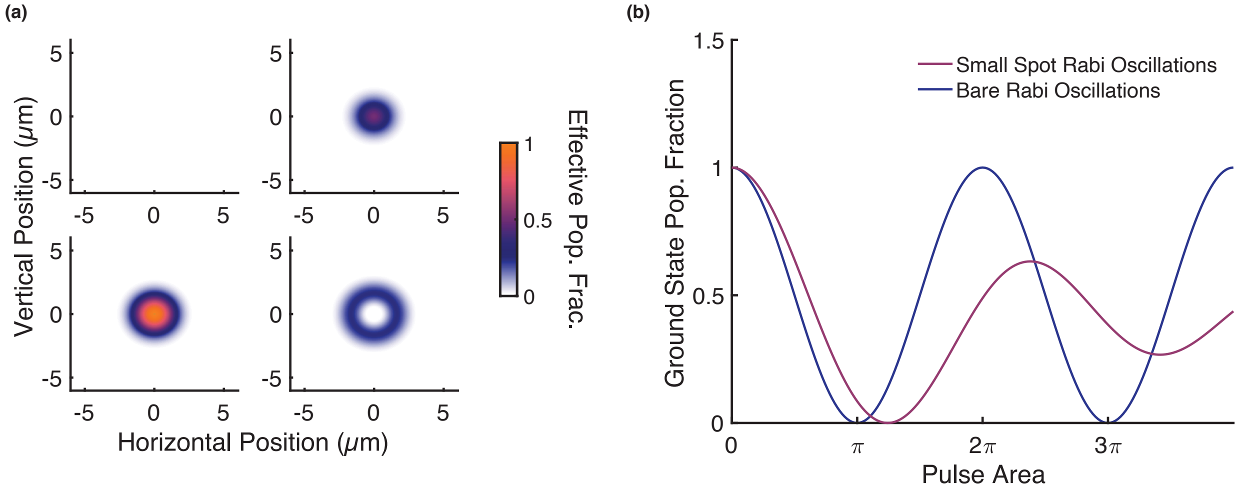


FIG. 5. The simulated ground state population at a pulse area of $0$,$\pi/2$,$\pi$, and $2\pi$ showing the spatial inhomogenaiety of the at-center pump field.

What is apparent from Figure 5(a) is that,as the pulse area increases, the Rabi flopping behavior spreads in an annular ring centered around the pump intensity maximum. As this happens, the apparent Rabi frequency is reduced as the center and wings of the distribution become more out of synch with eachother. However, the flopping behavior overall is not washed out. If we fit the simulated small-spot curve in Figure 5(b), we find an apparent

reduction in the Rabi frequency such that $\Omega_{apparent} = \text{b}\Omega_{real}$ with b = 0.81 estimated using the first minimum of the numerical simulation in 5(d), or b = 0.83 for a fit of the first three cycles of the numerical simulation to a damped oscillation with a finite offset. We will use the 'worse' value of b = 0.81 for our remaining calculation of $P_{\pi,thy}$.

Finally, to compare our fit to the *actual* $\pi$-pulse power we can calculate from the literature value of the dipole moment, we calculate the peak power required to flop a single center into the excited state, given a Gaussian electric field of waist $w_0$. Because the details of the calculation matter, we've outlined the basic but crucial derivation below. We start with the electric field

$$E(r,\theta) = E_0 \, e^{\frac{-r^2}{w_0^2}} . \tag{15}$$

Furthermore, assuming a Gaussian time-domain profile, we get that the field of a pi-pulse is

$$E_\pi = \frac{\hbar\pi}{\sqrt{2\pi}\mu_r\sigma} \tag{16}$$

Where we've used $\mu_r = \mu\sqrt{2} * b$ with b = 0.81 to correct for the inclination of the transition dipole moment of interest which is at an angle of 45° relative to the incident electric field and it's apparent reduction because of the finite pump size. We take $\sigma = 87$ fs for our measured pulse width, extracted from an auto-correlation of the FWM pulses. We then have that

$$P_{\pi,thy,peak} = \int_0^\infty \int_0^{2\pi} r \; d\theta \; dr \frac{c\epsilon(E_\pi)^2}{2} e^{\frac{-2r^2}{w_0}} \tag{17}$$

and thus

$$P_{\pi,thy,peak} = \frac{\pi^2 c\epsilon\hbar^2 w_0^2}{8\mu_r^2\sigma^2}. \tag{18}$$

When evaluated, we find that $P_{\pi,thy,peak} = 711$ W which, accounting for a pulse FWHM duration of 200 fs, and a repetition of 75.5 MHz yields $P_{\pi,thy} = 11.4$ mW. One final detail is that, to calculate $P_{\pi,exp}$, we take the true fit value and correct it for the index of refraction difference between vacuum and the diamond lattice, and the same 45° angle between the dipole moment and the effective field inside the diamond such that $P_{\pi,exp} = (0.5667/\sqrt{2}) * P_{\pi,fit} = 9.6$ mW as reported in the main text.

* Email: cundiff@umich.edu

[1] L. J. Rogers, K. D. Jahnke, M. W. Doherty, A. Dietrich, L. P. McGuinness, C. Müller, T. Teraji, H. Sumiya, J. Isoya, N. B. Manson, and F. Jelezko, Phys. Rev. B **89**, 1 (2014).

[2] C. Smallwood, T. Autry, and S. Cundiff, J. Opt. Soc. Am. B **34** (2016).
